# Supplementary material for: On the Ratio of Shannon Numbers of Graphs
Source: arXiv:2307.06155 source file (2024-12-09)
Supplement: Supplementary file 1 [file 8-Appendix.tex]

\section*{Appendix A}
\subsection{Generalized Independence Number of a graph}

\begin{definition}
For a graph $G$ and an integer $k$, we define $\alpha_k(G)$ as the maximum number of vertices that can be selected from $G$ such that, from any clique in $G$, at most $k$ vertices are chosen. It is important to note that a vertex may be selected multiple times.
\end{definition}

\begin{remark}
You can see that if $k = 1$, the above definition is the same as the normal independence number of a graph.
\end{remark}

\begin{remark}
\label{remark:frac}
If we define $\alpha_{k}^{*}$ similar to the fractional packing number, then we have $\alpha_{k}^{*}(G) = k \alpha^{*}(G)$ because the linear program to compute $\alpha_{k}^{*}(G)$ is basically $k$ times the linear program to calculate $\alpha^{*}(G)$.
\end{remark}

Note that Remark \ref{remark:frac} does not hold for the integral version, meaning that we don't necessarily have equality in $\alpha_{k}(G) \geq k \alpha(G)$. A counterexample for this equality occurs when $k = 2$ and $G = C_5$. In this case, we have $2 \cdot \alpha(C_5) = 4$, but $\alpha_{2}(C_5) = 5$.

\begin{theorem}
The generalized independence number is superadditive, meaning that for a graph $G$ and two integral numbers $k_1$ and $k_2$, we have $\alpha_{k_1}(G) + \alpha_{k_2}(G) \leq \alpha_{k_1 + k_2}(G)$.
\end{theorem}

\begin{proof}
It is easy to see because if $x$ is a solution to the integer program for finding $\alpha_{k_1}(G)$ and $y$ is a solution to the integer program for finding $\alpha_{k_2}(G)$, then $x+y$ is a solution to the integer program for finding $\alpha_{k_1 + k_2}(G)$.
\end{proof}

Now, we can show that we can calculate the fractional packing number using the generalized version of the independence number.
\begin{theorem}
\label{thm:ineq}
We have $\alpha_{k}(G \boxtimes W) \leq \alpha^{*}(G) \alpha_{k}(W)$.
\end{theorem}

\begin{proof}
The relaxed linear program for calculating the fractional packing number is given by:
\begin{equation}
\label{LP:genfrac}
\begin{array}{lll}
\text{maximize } & \sum\limits_{u \in V} x_{u} \\
\text{subject to } & \sum\limits_{u \in C} x_{u} \leq 1 \quad \forall \, \, Clique \, \, C \\
            & x \geq 0
\end{array}
\end{equation}
Let $A$ be a maximum $k$-generalized independent set in $G \boxtimes W$. For a vertex $u \in G$, we define $A_u$ as the projection of $A$ onto vertex $u$, i.e., $A_u = {v \in W \,|\, (u,v) \in A}$. It can be easily seen that $A_u$ is still a $k$-generalized independent set, and for a set of vertices in a clique $C$ in $G$, the union of their projections is also a $k$-generalized independent set.

Now, let us set $x_v = \frac{|A_u|}{\alpha_{k}(W)}$ for all vertices $v$ in $W$. By the above arguments, we can conclude that $x$ is a feasible solution for LP \ref{LP:genfrac}. Hence, we have:
\[
\sum\limits_{u \in V} x_{u} = \sum\limits_{u \in V} \frac{|A_u|}{\alpha_{k}(W)} = \frac{\alpha_{k}(G \boxtimes W)}{\alpha_{k}(W)} \leq \alpha^{*}(G)
\]
Thus, we have shown that $\alpha_{k}(G \boxtimes W) \leq \alpha^{*}(G) \alpha_{k}(W)$, as desired.
\end{proof}
\begin{remark}
\label{remark:enqu}
If we set $W$ to be a graph with a single vertex, then the above inequality says that $\alpha_{k}(G) \leq k \alpha^{*}(G)$.
\end{remark}

\begin{theorem}
$\sup\limits_{W} \frac{\alpha_{k}(G \boxtimes W)}{\alpha_{k}(W)} = \alpha^{*}(G)$.
\end{theorem}

\begin{proof}
Based on Theorem \ref{thm:ineq}, we have one side of the inequality. For the other side, we need to show that there exists a graph $W$ for which equality holds. Let $x^{*}$ be the optimal solution to LP \ref{LP:genfrac}, and let $N$ be a large integer such that for any vertex $i \in G$, the number $n_i := x^{*}_{i}N$ is an integer.

Consider the graph $W = G^{c}(n_1, n_2, \dots, n_{|V|})$ where each vertex $u_i$ is repeated $n_i$ times. We claim that this graph maximizes the expression $\frac{\alpha_{k}(G \boxtimes W)}{\alpha_{k}(W)}$, and equality holds for this graph.

To find $\alpha_{k}(G \boxtimes W)$, we can pick vertex $u$ $n_u$ times. Since for any clique $C$, we have:
\[
\sum\limits_{u \in C} n_{u} = N \sum\limits_{u \in C} x^{*} \leq N
\]
This new set is a feasible solution for $\alpha_{k}(G \boxtimes W)$, and its value is the following:
\[\sum\limits_{u \in V} n_{u} = N \sum\limits_{u \in V} x^{*} = N \alpha^{*}(G)\]
By Remark \ref{remark:enqu}, this is the optimal solution and we have shown that $\sup\limits_{W} \frac{\alpha_{k}(G \boxtimes W)}{\alpha_{k}(W)} = \alpha^{*}(G)$.
\end{proof}

\begin{theorem}
\label{thm:oneN}
For any graph $G$, there exists an integer $k$ such that $\alpha_{k}(G) = k \alpha^{*}(G)$.
\end{theorem}

\begin{proof}
Define $x^{*}$ and $N$ as in the previous theorem. By the previous inequalities it is trivial that we have $\alpha_{N}(G) = N \alpha^{*}(G)$. Hence, we have shown that for any graph $G$, there exists an integer $k$ such that $\alpha_{k}(G) = k \alpha^{*}(G)$.
\end{proof}
\begin{theorem}
For a collection of graphs $G_1, \dots , G_k$, there exists an integer $k$ such that for every $i$, $\alpha_{k}(G_i) = k \alpha^{*}(G_i)$.
\end{theorem}

\begin{proof}
Using Theorem \ref{thm:oneN} and the superadditivity of the generalized independent number, we can see that if we set $k = N_1 \times \dots \times N_k$, where $N_i$ is a large integer such that multiplying the optimal solution of the LP for graph $G_i$ by $N_i$ gives an integer answer, then we have the desired property.
\end{proof}

\begin{theorem}
For any graph $G$, we have $\lim\limits_{n \to \infty} \frac{\alpha_{n}(G)}{n} = \alpha^{*}(G)$.
\end{theorem}

\begin{proof}
First, set $N$ to be the large number for which Theorem \ref{thm:oneN} holds. Now, consider a number $M = Nq + r$, where $q, r \in \mathbb{N}$ and $r < N$. By the superadditivity of the generalized independence number, we have $(M-N) \alpha^{*}(G) \leq qN \alpha^{*}(G) \leq qN \alpha^{*}(G) + \alpha_{r}(G) \leq \alpha_{M}(G)$. Additionally, using Remark \ref{remark:enqu}, we have $\alpha_{M}(G) \leq M \alpha^{*}(G)$.

Now, we can conclude that:
\begin{equation*}
\lim\limits_{n \to \infty} \frac{(n-N) \alpha^{*}(G)}{n} \leq \lim\limits_{n \to \infty} \frac{\alpha_{n}(G)}{n} \leq \lim\limits_{n \to \infty} \frac{n \alpha^{*}(G)}{n}
\end{equation*}
Since $N$ is a constant, we can simplify further and state that $\lim\limits_{n \to \infty} \frac{\alpha_{n}(G)}{n} = \alpha^{*}(G)$. Thus, the theorem is proved.

The similarity of the above theorem with the definition of the fractional chromatic number is really interesting. If we take the dual of the integer program used to calculate the $k$-generalized independent number of a graph $G$, it corresponds to covering the vertices of $G$ with cliques such that each vertex is covered by at least $k$ cliques. If we assign different colors to each vertex in different cliques, it becomes a $k$-fold coloring of the vertices of $G^c$, which is one of the ways we define the fractional chromatic number.
\end{proof}
